# Supplementary material for: FastSeq: Make Sequence Generation Faster
Source: arXiv:2106.04718 source file (2021-07-12)
Supplement: Supplementary file 1 [file acl2021_appendix.tex]

%
% File acl2021.tex
%
%% Based on the style files for EMNLP 2020, which were
%% Based on the style files for ACL 2020, which were
%% Based on the style files for ACL 2018, NAACL 2018/19, which were
%% Based on the style files for ACL-2015, with some improvements
%%  taken from the NAACL-2016 style
%% Based on the style files for ACL-2014, which were, in turn,
%% based on ACL-2013, ACL-2012, ACL-2011, ACL-2010, ACL-IJCNLP-2009,
%% EACL-2009, IJCNLP-2008...
%% Based on the style files for EACL 2006 by 
%%e.agirre@ehu.es or Sergi.Balari@uab.es
%% and that of ACL 08 by Joakim Nivre and Noah Smith

\documentclass[11pt,a4paper]{article}
\usepackage[hyperref]{acl2021}
\usepackage{times}
\usepackage{latexsym}

% This is not strictly necessary, and may be commented out,
% but it will improve the layout of the manuscript,
% and will typically save some space.
\usepackage{microtype}

% begin add package
\usepackage{amsmath}
\usepackage{pgf-pie}
\usepackage{algorithm}
\usepackage{algorithmic}
% end add package

\aclfinalcopy % Uncomment this line for the final submission
%\def\aclpaperid{} %  Enter the acl Paper ID here

%\setlength\titlebox{5cm}
% You can expand the titlebox if you need extra space
% to show all the authors. Please do not make the titlebox
% smaller than 5cm (the original size); we will check this
% in the camera-ready version and ask you to change it back.

\title{Appendix for FastSeq – Make Sequence Generation Faster}

\begin{document}
%\maketitle

\appendix

\input{appendix}

\end{document}
